# Supplementary material for: MixRec: Heterogeneous Graph Collaborative Filtering
Source: arXiv:2412.13825 source file (2024-12-25)
Supplement: Supplementary file 1 [file appendix.tex]

\section{Appendix}
